# Supplementary material for: Adaptive Bounded Exploration and Intermediate Actions for Data Debiasing
Source: arXiv:2504.08151 source file (2025-04-10)
Supplement: Supplementary file 1 [file related-additional.tex]

\section{Additional and Detailed Related Work}\label{app:related-additional}

\textbf{Interplay of fairness criteria and data biases.} Our analysis in Section~\ref{sec:two-group}, similar to those of \citet{blum2020recovering} and \citet{jiang2020identifying}, also considers the interplay between algorithmic fairness rules and data biases. \citet{blum2020recovering} show that certain fairness constraints can \emph{themselves} be interpreted as enabling debaising of the underlying estimates. Also, both works 
study data bias arising due to the \emph{labeling} process and propose reweighting techniques to address it. Our work differs from these from two main aspects. First, we model biases as changes in feature-label distributions, in contrast to the assumption of noisy labels in these works. Second, we introduce a statistical debiasing technique based primarily on exploration, which is orthogonal to the social debiasing achieved through fairness constraints. Our proposed model and algorithm therefore complement these works. 

\textbf{Long-term fairness and bias in algorithmic decision making:} The majority of works on fair algorithmic decision making have focused on achieving fairness in a one-shot setting (i.e. without regards to the long-term effects of the proposed algorithms); see e.g.~\citep{hardt2016equality,dwork2012fairness,corbett2017algorithmic}. Some recent works have studied long-term impacts of fairness on disparities, group representation, and strategic manipulation of features, as a result of adopting fairness measures~\citep{liu2018delayed,zhang2019group,liu2020disparate}. Our work contributes to this line of research, by analyzing the long-term effects of imposing fairness constraints on data collection and debiasing efforts. 

\textbf{Biases in adaptively collected data:} A few other works have, similar to our work, explored the question of biases induced by a decision rule on data collection. \citet{deshpande2018accurate} study inference in a linear model with adaptively collected data; in contrast to our proposed method, their work focuses on debiasing of an estimator, rather than modifying the decision rule used to collect the data.  \citet{nie2018adaptively} study the problem of estimating statistical parameters from adaptively collected data. Their proposed adaptive data collection method, which also similar to ours (Assumption~\ref{as:distributions}) is used for single-parameter estimation, is one of online debiasing; our proposed data collection methods however differ. In particular, our focus is on accounting for multiple subgroups as well as fairness considerations. More importantly, we propose a \emph{bounded} exploration strategy, which accounts for the risks of exploration decisions and limits the depth of exploration; this method of exploration is different from the random exploration used to collect the data in~\citep{nie2018adaptively}, to which their proposed debiasing algorithms based on data splitting and modified maximum likelihood estimators are applied.  

\textbf{Active learning}: Our work is also related to the active learning literature. \citet{balcan2007margin} study the sample complexity of labeled data required for active learning, \citet{kazerouni2020active} propose an algorithm involving exploration and exploitation-based adaptive sampling, verifying it using simulations, \citet{abernethy2022active} propose an active sampling and re-weighting technique by sampling from the worst off group at each step with the goal of building a computationally efficient algorithm with strong convergence guarantees to improve the performance on the disadvantage (highest loss) group while satisfying the notion of min-max fairness, \citet{noriega2019active} propose an adaptive fairness approach, which adaptively acquires additional information according to the needs of different groups or individuals given information budgets, to achieve fair classification. Similar to the approaches of these papers, we also compensate for adaptive sampling bias through exploration (by admitting individuals who would otherwise be rejected). Comparing to all these literature, we start with a biased dataset, and we primarily focus on recovering the true distribution by bounded exploration, accounting for the cost of exploration, avoiding the adaptive sampling bias, and consider fairness issues as orthogonal to our data collection procedure (and as such, can apply our procedure to debiasing the estimates on a single group). 

\textbf{Selective labeling bias}: \citet{lakkaraju2017selective} address the problem of evaluating the performance of predictive model under the selective labeling problem. They propose a contraction technique to compare the performance of the predictive model and human judge while they are forced to have the same acceptance rate. \citet{de2018learning} study the problems arising due to selective labeling. Similar to us, they propose a data augmentation scheme by adding more samples that would be more likely rejected (we refer to this as exploration) to correct the sample selection bias. Their proposed data augmentation technique is similar to our bounded exploration, but it differs in its selection of samples in that it adds samples that would be more likely to be rejected. 

\textbf{Fair learning}: \citet{kallus2018residual} show that residual unfairness remains even after the adjustment for fairness when policies are learned from a biased dataset. They propose a re-weighting technique (similarly, re-weighing ideas are explored in \citep{blum2020recovering} and \citep{jiang2020identifying}) to solve the residual unfairness issue while accounting for the censoring/adaptive sampling bias. 

\textbf{Online mean estimation:} Compared to this literature, the main technical challenges of our proposed bounded exploration in online mean estimation is that it involves evaluating the behavior of statistical estimates based on data collected from a truncated distribution with \emph{time-varying} truncation. More specifically, our data collection interval is bounded and truncated (which has been considered in some prior work on distribution/mean estimation as well, e.g., \citet{lai1991estimating}) but our exploration interval $[LB_t, \infty)$ is itself adaptive (which we believe is the main new aspect) and is what has motivated our analysis in a finite sample regime in Theorem 3. Our focus on the interplay of fairness constraints with online estimation efforts (Proposition 1) is also new compared to this existing literature.

\textbf{Performative prediction:} Finally, the recent line of work on performative prediction proposed by \citet{perdomo2020performative}  also considers the effects of algorithmic decisions on the underlying population's features-label distributions. In particular, the choice of the ML model can cause a shift in the data distribution, and the goal of this work is to identify the stable ML model parameter that is attained at a fixed point of the algorithm-population interactions. In contrast, our focus is on \emph{pre-existing} and unchanging distribution shifts in the data, which our \texttt{active debiasing} algorithm aims to correct over time. Therefore, our algorithm could be considered as a debiasing method to be used when such performative shifts are present in the data, but are unaccounted for: If distribution shifts happen relatively slower than our debiasing algorithm's convergence speed, our \texttt{active debiasing} could be used to recover correct estimates of the underlying distribution, the estimates of which might be biased due to performative distribution shifts.
